# Supplementary material for: Ultrafast coherent all-optical switching of an antiferromagnet with the inverse Faraday effect
Source: arXiv:2104.11820 ancillary file (2021-08-08)
Supplement: Supplementary file 1 [file supplemental.pdf]

## Supplemental material

# Ultrafast coherent all-optical switching of an antiferromagnet with the inverse Faraday effect

Tobias Dannegger[1], Marco Berritta[2], Karel Carva[3], Severin Selzer[1], Ulrike Ritzmann[2,4], Peter M. Oppeneer[2], and Ulrich Nowak[1]

[1]*Fachbereich Physik, Universität Konstanz, D-78457 Konstanz, Germany*
[2]*Department of Physics and Astronomy, Uppsala University, Box 516, SE-75120 Uppsala, Sweden*
[3]*Charles University, Faculty of Mathematics and Physics, Department of Condensed Matter Physics, Ke Karlovu 5, CZ-121 16 Prague, Czech Republic*
[4]*Dahlem Center of Complex Quantum Systems and Department of Physics, Freie Universität Berlin, Arnimallee 14, D-14195 Berlin, Germany*

## Contents

**1 Implementation details of the atomistic spin dynamics simulations 2**
1.1 Formulation of Hamiltonian, effective field and LLG equation . . 2
1.2 Renormalization of the saturation moment . . . . . . . . . . . . . 3
1.3 Two-temperature model . . . . . . . . . . . . . . . . . . . . . . . 4
1.4 Induced magnetic moments resolved by atom type . . . . . . . . . 5

**2 Influence of various parameters on switching probabilities 6**
2.1 Temperature and heating . . . . . . . . . . . . . . . . . . . . . . . 6
2.2 Antiferromagnetic vs. ferrimagnetic order . . . . . . . . . . . . . 8
2.3 Gilbert damping parameter . . . . . . . . . . . . . . . . . . . . . . 10
2.4 Decay time of the induced moments . . . . . . . . . . . . . . . . . 12

# 1 Implementation details of the atomistic spin dynamics simulations

## 1.1 Formulation of Hamiltonian, effective field and LLG equation

As stated in the main text, we incorporate the induced magnetic moments into the spin model by replacing the atomic spin vector $\boldsymbol{S}_i$ by the total spin vector $\boldsymbol{S}_{i,\mathrm{tot}} := \boldsymbol{S}_i + \Delta\boldsymbol{S}_i = (\boldsymbol{\mu}_i + \boldsymbol{\mu}_{i,\mathrm{ind}})/\mu_s$ in the Hamiltonian. This total spin vector does not have a conserved length, as it is still normalized to $\mu_s$. Compared with a normalization to the total magnetic moment, $(\boldsymbol{\mu}_i + \boldsymbol{\mu}_{i,\mathrm{ind}})/\mu_{i,\mathrm{tot}}$, this can be seen as a result of the approximation $\mu_{i,\mathrm{tot}} \approx \mu_s$ (cf. Sec. 1.2). If we write out the resulting modified Hamiltonian, we get the following expression:

$$
\begin{aligned}
\mathscr{H} &= -\sum_{i\neq j} J_{ij}\boldsymbol{S}_{i,\mathrm{tot}}\cdot\boldsymbol{S}_{j,\mathrm{tot}} - \sum_i \left[d_z S_{i,\mathrm{tot},z}^2 + 4d_{\mathrm{ip}} S_{i,\mathrm{tot},x}^2 S_{i,\mathrm{tot},y}^2\right] \\
&= -\sum_{i\neq j} J_{ij}(\boldsymbol{S}_i + \Delta\boldsymbol{S}_i)\cdot(\boldsymbol{S}_j + \Delta\boldsymbol{S}_j) \\
&\quad - \sum_i \left[d_z(S_{i,z} + \Delta S_{i,z})^2 + 4d_{\mathrm{ip}}(S_{i,x} + \Delta S_{i,x})^2(S_{i,y} + \Delta S_{i,y})^2\right] \\
&= -\sum_{i\neq j} J_{ij}\boldsymbol{S}_i\cdot\boldsymbol{S}_j - \sum_i d_z S_{i,z}^2 - \sum_i 4d_{\mathrm{ip}} S_{i,x}^2 S_{i,y}^2 \\
&\quad - \sum_{i\neq j} J_{ij}\Delta\boldsymbol{S}_i\cdot\Delta\boldsymbol{S}_j - \sum_i d_z \Delta S_{i,z}^2 - \sum_i 4d_{\mathrm{ip}}\Delta S_{i,x}^2\Delta S_{i,y}^2 \\
&\quad - \sum_{i\neq j} 2J_{ij}\boldsymbol{S}_i\cdot\Delta\boldsymbol{S}_j - \sum_i 2d_z S_{i,z}\Delta S_{i,z} \\
&\quad - \sum_i 4d_{\mathrm{ip}}\big[S_{i,x}^2\Delta S_{i,y}^2 + S_{i,y}^2\Delta S_{i,x}^2 + 4S_{i,x}S_{i,y}\Delta S_{i,x}\Delta S_{i,y} \\
&\qquad + 2S_{i,x}\Delta S_{i,x}\big(S_{i,y}^2 + \Delta S_{i,y}^2\big) + 2S_{i,y}\Delta S_{i,y}\big(S_{i,x}^2 + \Delta S_{i,x}^2\big)\big]. \qquad \text{(S1)}
\end{aligned}
$$

In the last step, we sorted the terms into an atomic part (first line), which is equivalent to the unmodified Hamiltonian, a mathematically equivalent set of terms for the induced moment (second line), and the remaining mixed terms. The

effective field is now given by the negative gradient of $\mathscr{H}$ with respect to $\boldsymbol{S}_i$[1]:

$$\boldsymbol{H}_i = -\frac{\mathrm{d}\mathscr{H}}{\mathrm{d}\boldsymbol{S}_i} + \boldsymbol{\zeta}_i(t) = -\frac{\partial\mathscr{H}}{\partial\boldsymbol{S}_{i,\mathrm{tot}}}\frac{\mathrm{d}\boldsymbol{S}_{i,\mathrm{tot}}}{\mathrm{d}\boldsymbol{S}_i} + \boldsymbol{\zeta}_i(t)$$
$$= 2\sum_j J_{ij}(\boldsymbol{S}_j + \Delta\boldsymbol{S}_j) + 2d_z(S_{i,z} + \Delta S_{i,z})\boldsymbol{e}_z + 8d_{\mathrm{ip}}\begin{pmatrix} (S_{i,x} + \Delta S_{i,x})(S_{i,y} + \Delta S_{i,y})^2 \\ (S_{i,x} + \Delta S_{i,x})^2(S_{i,y} + \Delta S_{i,y}) \\ 0 \end{pmatrix} + \boldsymbol{\zeta}_i(t) \tag{S2}$$

with a thermal noise $\boldsymbol{\zeta}_i(t)$ that satisfies the conditions

$$\langle\boldsymbol{\zeta}_i(t)\rangle = 0, \quad \langle\zeta_{i,\eta}(t)\zeta_{i,\theta}(t')\rangle = \delta_{ij}\delta_{\eta\theta}\delta(t-t')\frac{2\alpha\mu_s}{\gamma}k_B T \tag{S3}$$

where $\eta, \theta \in \{x, y, z\}$ are the Cartesian coordinates, $k_B$ is the Boltzmann constant and $T$ the temperature. In the simulations, we use pseudo-random numbers with a Gaussian distribution for this noise term. Note that in Eq. (S2) we used $\mathrm{d}\boldsymbol{S}_{i,\mathrm{tot}}/\mathrm{d}\boldsymbol{S}_i = \mu_s/\mu_{i,\mathrm{tot}} = 1$, as we neglect the change of the total magnetic moment in our approximation. The resulting effective field therefore has the same form as it would without induced moment, except that the spin $\boldsymbol{S}_i$ is replaced by $\boldsymbol{S}_{i,\mathrm{tot}} = \boldsymbol{S}_i + \Delta\boldsymbol{S}_i$. With this effective field, we can use the LLG equation in its known form:

$$\frac{\mathrm{d}}{\mathrm{d}t}\boldsymbol{S}_i = -\frac{\gamma}{1+\alpha^2}\frac{1}{\mu_s}\boldsymbol{S}_i \times (\boldsymbol{H}_i + \alpha\boldsymbol{S}_i \times \boldsymbol{H}_i). \tag{S4}$$

Note that even though the Hamiltonian was formulated for the total magnetic moment, we computed the effective field and the LLG equation for the atomic spin $\boldsymbol{S}_i$ and not the sum $\boldsymbol{S}_i + \Delta\boldsymbol{S}_i$.

## 1.2 Renormalization of the saturation moment

The action of the IFE leads to a small reduction of the saturation moments $\mu_s$ that occurs briefly during the laser pulse because of the induced magnetic moments. Instead of $\mu_s = |\boldsymbol{\mu}_i|$ (note that $|\boldsymbol{\mu}_i|$ is the same for all lattice sites), the magnetic moment of the lattice site can be written as $\mu_{s,i} = |\boldsymbol{\mu}_i + \boldsymbol{\mu}_{\mathrm{ind},i}|$ (now lattice site-dependent) in the presence of an induced magnetic moment. Since this change amounts to less than 1 %, even at the peak of the laser pulse, it does not influence the dynamics in any significant way. To check this assumption, we repeated the same longitudinal switching simulations renormalizing the saturation moments at

[1]The effective field may also be defined as $-\partial\mathscr{H}/\partial\boldsymbol{\mu}_i = -(\partial\mathscr{H}/\partial\boldsymbol{S}_i)(\partial\boldsymbol{S}_i/\partial\boldsymbol{\mu}_i) = -(1/\mu_s)(\partial\mathscr{H}/\partial\boldsymbol{S}_i)$. With this definition, the prefactor $1/\mu_s$ would not appear in the LLG equation.

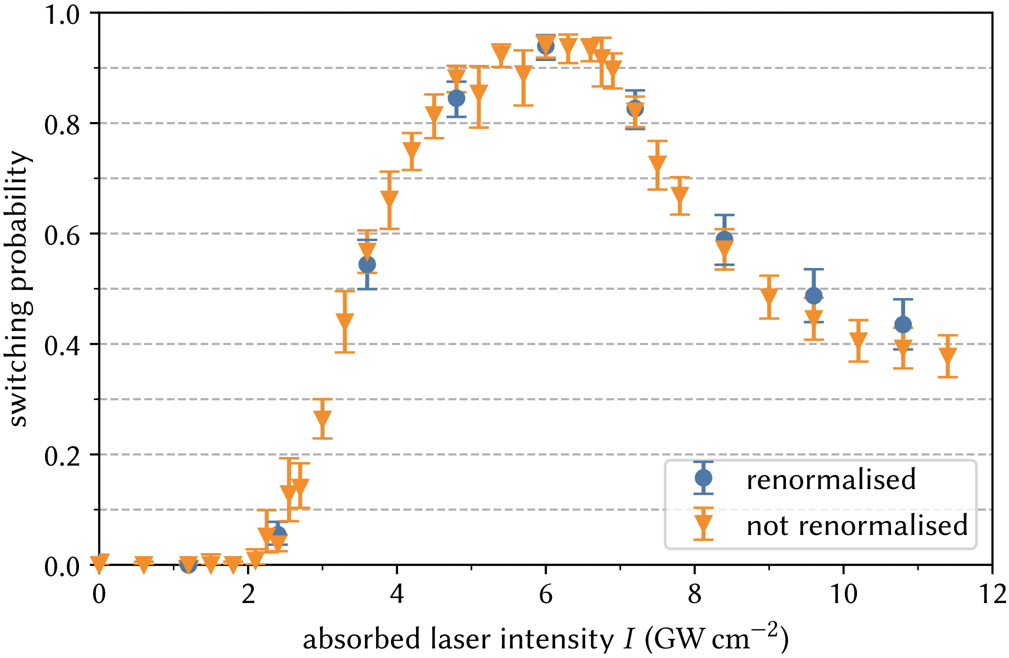


Figure S1: Simulated switching probabilities with and without renormalization of the saturation moments. The error bars indicate the 95 % confidence interval.

every timestep. As expected, Fig. S1 shows that the renormalization does not lead to any measurable difference in the results.

In addition, we can conclude from Fig. S7, see Sec. 2.2, that even a permanent change of the saturation moment of a few percent would not change the results measurably.

### 1.3 Two-temperature model

The temperature evolution in our model is described by a simple two-temperature model. The power of the laser pulse $P(t)$ is first absorbed by the electronic subsystem with temperature $T_{\mathrm{el}}$ and heat capacity $C_{\mathrm{el}} = \gamma_{\mathrm{el}} T_{\mathrm{el}}$ where $\gamma_{\mathrm{el}} = 88.3\,\mathrm{J\,K^{-2}\,m^{-3}}$ is the Sommerfeld coefficient. The Sommerfeld coefficient depends on the density of states at the Fermi level which we have extracted from the DFT calculations. Heat from the electrons is then transferred to the phonon heat bath with temperature $T_{\mathrm{ph}}$ and heat capacity $C_{\mathrm{ph}} = 3nk_B = 2.98\,\mathrm{MJ\,K^{-1}\,m^{-3}}$ (in the Debye model). The rate of this heat transfer is quantified by the electron-phonon coupling constant $G = 4.0 \times 10^{17}\,\mathrm{W\,K^{-1}\,m^{-3}}$ (taken to be the same as for FePt, see Ref. [1]). The time

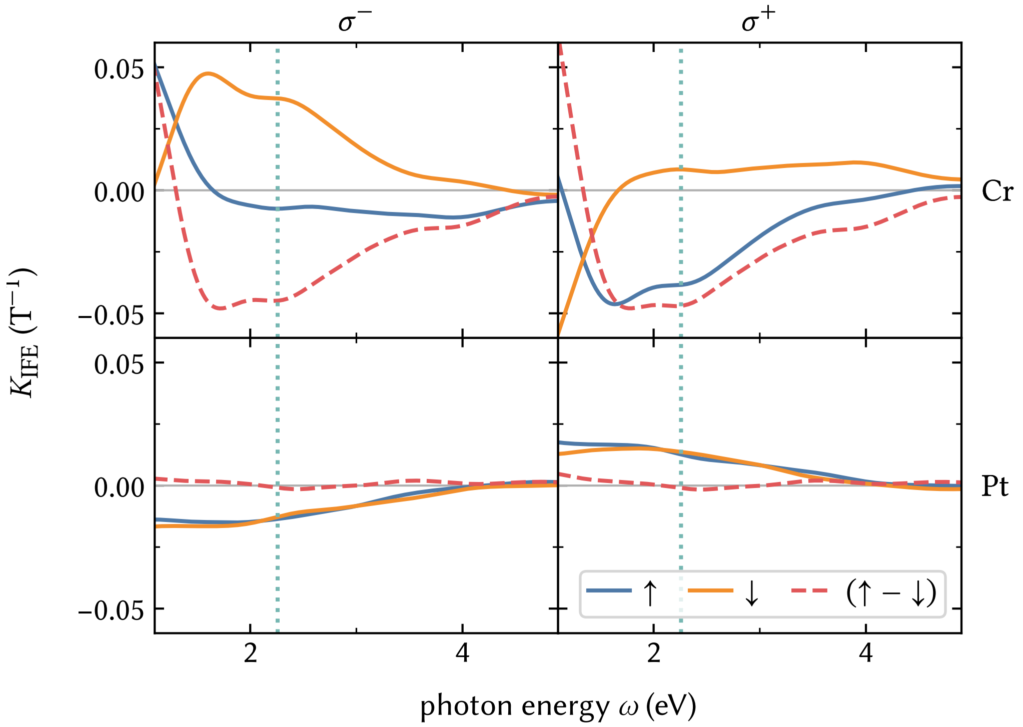


Figure S2: Ab initio computed IFE constants resolved by atom type, sublattice and helicity. The dotted turquoise line marks the photon energy used in the simulations.

evolution of those two temperatures is described by two coupled rate equations:

$$C_{\mathrm{el}}\dot{T}_{\mathrm{el}} = G(T_{\mathrm{ph}} - T_{\mathrm{el}}) + P(t), \tag{S5}$$

$$C_{\mathrm{ph}}\dot{T}_{\mathrm{ph}} = G(T_{\mathrm{el}} - T_{\mathrm{ph}}). \tag{S6}$$

The electronic temperature $T_{\mathrm{el}}$ is the one that enters into the LLG equation via the thermal noise field $\zeta$.

### 1.4 Induced magnetic moments resolved by atom type

Figure S2 shows the DFT-calculated IFE constants, resolved by atom type. On the Cr sites, the orientation of the local spin with respect to the $\boldsymbol{k}$-vector and the helicity of the incident light determines the sign and magnitude of the induced moment. In contrast, the Pt sites do not have an inherent magnetic moment breaking the symmetry, therefore the sign of the induced magnetic moments there only depends on the helicity of the light. Consequently, the staggered induced moment vanishes on the Pt sites. Therefore, the coupling of the Cr spins to the induced moments on Pt can be neglected because this would only decrease the effective moment on one

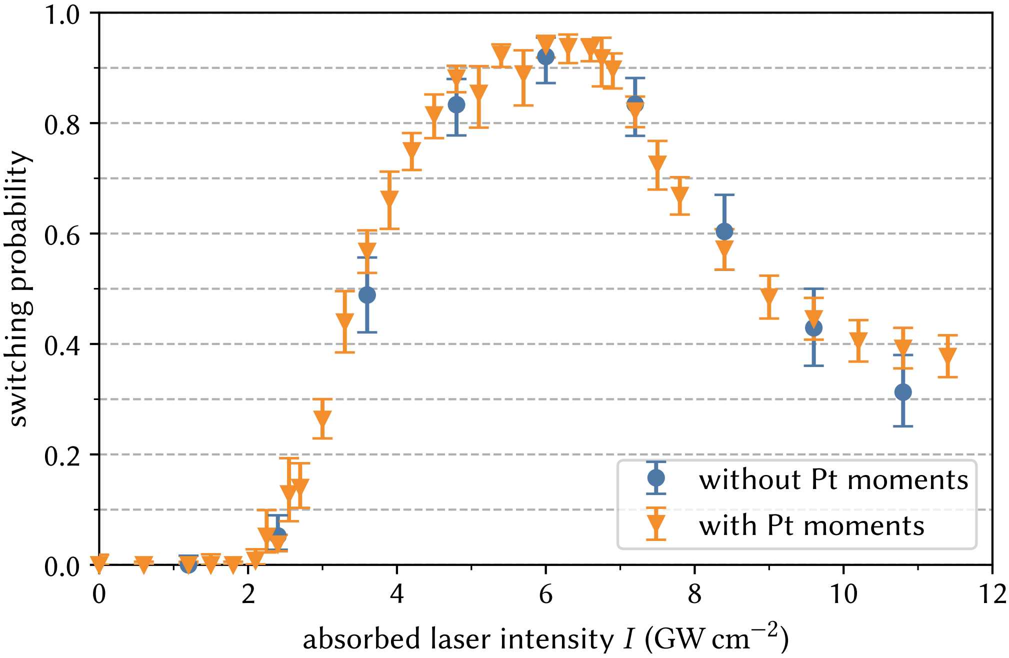


Figure S3: Simulated switching probabilities with and without taking the laser induced magnetic moments on Pt into account. The error bars indicate the 95 % confidence interval.

of the sublattices by the same amount that it increases the moment on the other sublattice. The staggered induced moment hence remains the same and therefore the dynamics do not change.

To test this conclusion, we repeated the simulations of the longitudinal switching process both without the induced moments on Pt (using only the moments induced on the Cr sites) and with the induced moments on Pt (assuming an equal contribution of both Cr and Pt induced moments). The results of these simulations can be seen in Fig. S3. For some intensity values, it looks as if the switching probability might decrease by a small amount without the induced moments on Pt, but the difference is too small to come to a clear conclusion about that. It does certainly not lead to any qualitative difference.

## 2 Influence of various parameters on switching probabilities

### 2.1 Temperature and heating

Figure S4 shows a more detailed analysis of how the laser-induced heating contributes to the switching probability by modulating the amount of power that enters

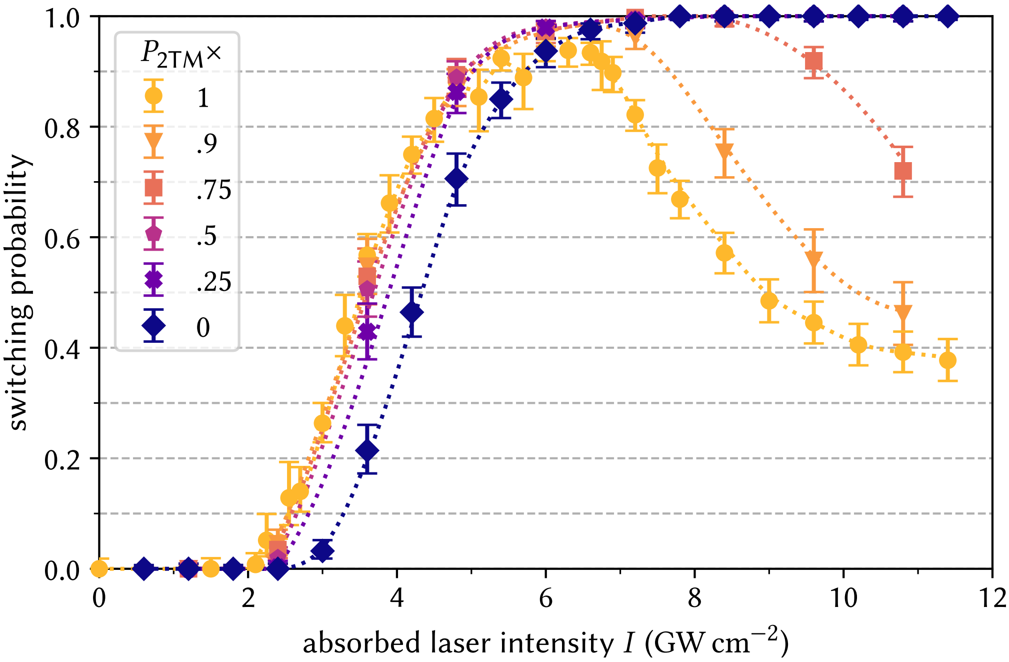


Figure S4: Simulated switching probabilities with reduced laser-induced heating. The dotted lines serve as a guide to the eye. The error bars indicate the 95 % confidence interval.

into the two-temperature model between 0 (no heating at all) and 1 (the realistic amount of heating), while leaving the induced magnetic moments at their normal values. The data show clearly that the heating of the material is not needed to obtain antiferromagnetic switching. On the contrary, at very high laser intensities, the strong heating of the material hinders the coherent switching process, since it reduces the switching probability by randomizing the magnetization. Without any heating, the switching probability would remain at 1 for high intensities. A certain amount of heating, however, makes the switching process slightly more efficient at lower intensities. This is why the graph for $P_{2TM} = 0$ is slightly lower below $I \approx 6\,\mathrm{GW\,cm^{-2}}$. Here, the additional thermal energy helps moving over the anisotropy barrier, but this effect is only marginal. Instead, the switching probability scales with the magnitude of the induced magnetic moment. This can be seen in Fig. S5, where the IFE constants have been modulated by a factor between 0 (no IFE) and 1 (original values from the DFT calculations). Dissipative effects randomize the magnetization for higher intensities, but controllable switching takes place at lower intensities where the thermal effects are insignificant. Dissipative effects should still be included in such simulations to give a realistic estimate of the achievable

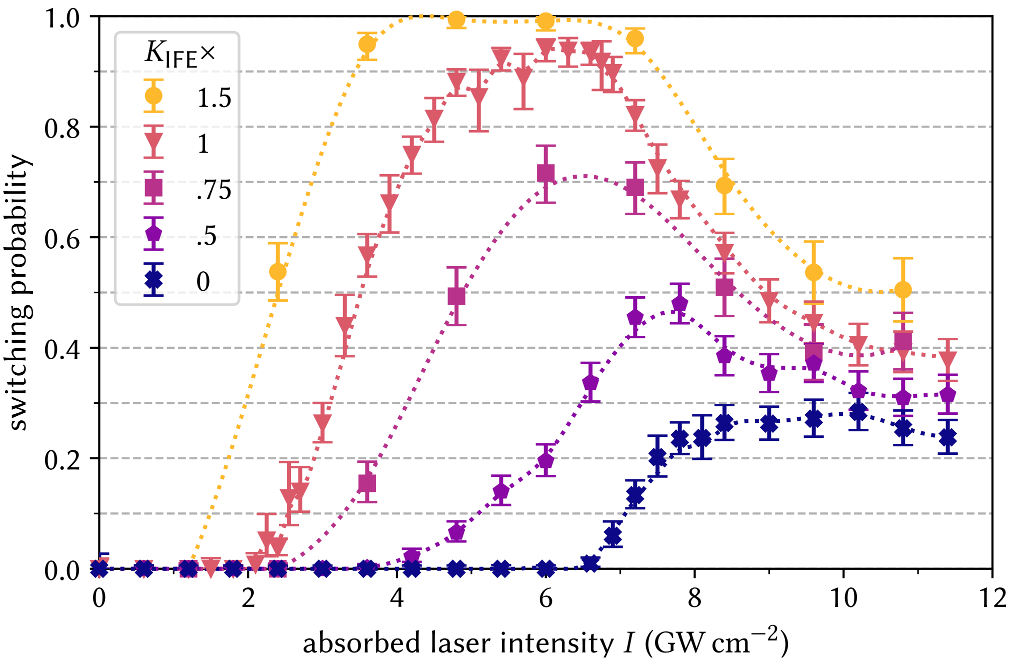


Figure S5: Simulated switching probabilities with varying IFE constants. The dotted lines serve as a guide to the eye. The error bars indicate the 95 % confidence interval.

switching probabilities, especially at higher laser intensities.

A finite initial temperature is also needed because, if the induced magnetic moments were perfectly parallel to the initial magnetization of the material (as they are in the ground state), there would be no torque acting on the spins. At room temperature, thermal fluctuations ensure there is an angle of a few degrees between the spins and the axis of the $\boldsymbol{k}$-vector. However, if we initialize the system with a finite angle between the magnetization axis and the $\boldsymbol{k}$-vector, the switching can still be observed at $T = 0$. Figure S6 shows an example of such simulations that were carried out without the stochastic term of the LLG. The process is deterministic in that case and the outcome depends on the initial angle and on the laser intensity.

### 2.2 Antiferromagnetic vs. ferrimagnetic order

In the main text, it was explained how the coherent switching in antiferromagnets is contingent on the particular properties of that type of magnetic order. In order to examine how different the magnetic moments of the sublattices can be (i.e., 'how ferrimagnetic' the material can be) without obstructing the switching, the magnetic moment of one of the sublattices was varied while keeping the other constant. The results of these simulations are presented in Fig. S7. They show that

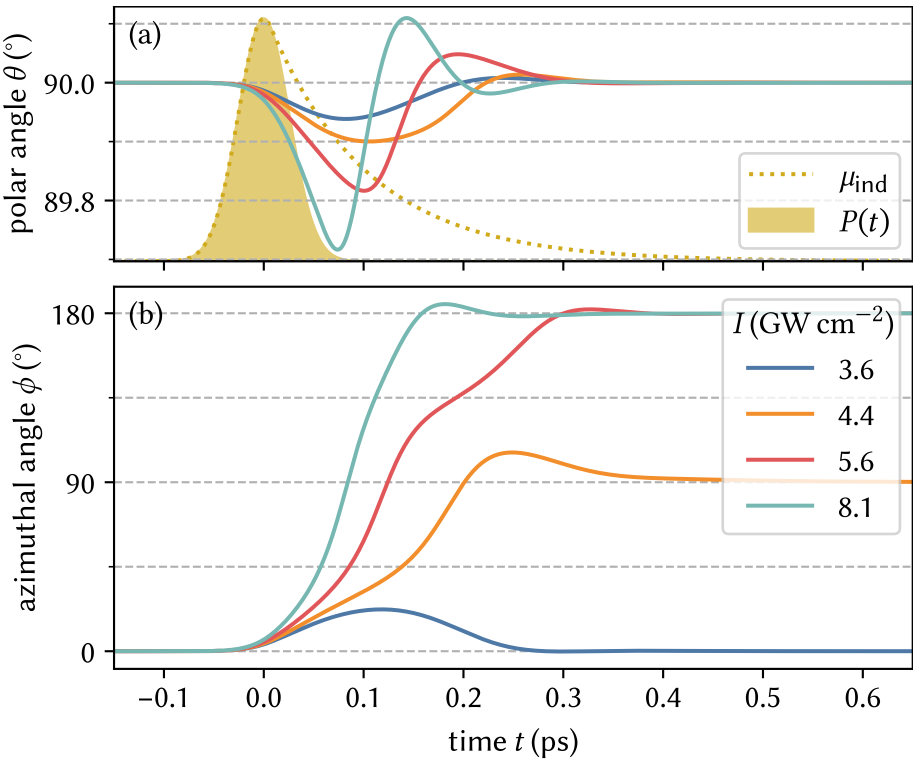


Figure S6: Time evolution of the spherical coordinates of the Néel vector in a switching simulation without the stochastic term. An angle of 2° was set between the initial magnetization and the $\boldsymbol{k}$-vector of the incident light.

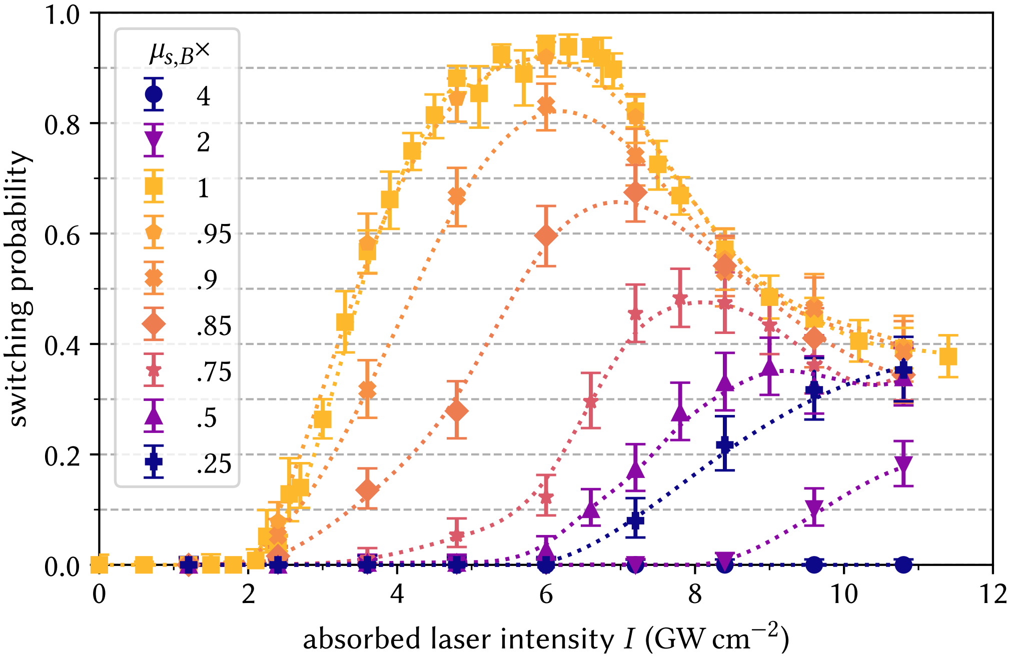


Figure S7: Simulated switching probabilities with unequal sublattice moments (i.e., with ferrimagnetic order). The dotted lines serve as a guide to the eye. The error bars indicate the 95 % confidence interval.

a small difference between the sublattices (one moment reduced to 95 %) does not reduce the switching probability significantly. At 90 % it begins to diminish and at 50 % it is almost completely suppressed. Despite the overall reduction of the system's magnetic moment, which according to the LLG leads to an acceleration of the dynamics and by itself should enhance the switching process, the asymmetry between the sublattices inhibits the switching process. (This reduction of the switching probability is even more pronounced if the magnetic moment is increased instead of decreased.) At 25 % (the same ratio as GdFeCo), the switching probability does not differ clearly from the pure thermal case without the IFE, consistent with previous results showing that switching in GdFeCo is thermally driven [2, 3].

### 2.3 Gilbert damping parameter

It was mentioned in the main text that the value of the Gilbert damping parameter $\alpha$ should realistically be around 0.05, i.e., similar to the values known for CoPt and FePt [4, 5]. But because the value for CrPt is not known exactly, it was varied in a wide range around that value to determine how it influences the switching probability, see Fig. S8. Unsurprisingly, the switching is enhanced for lower damping values and

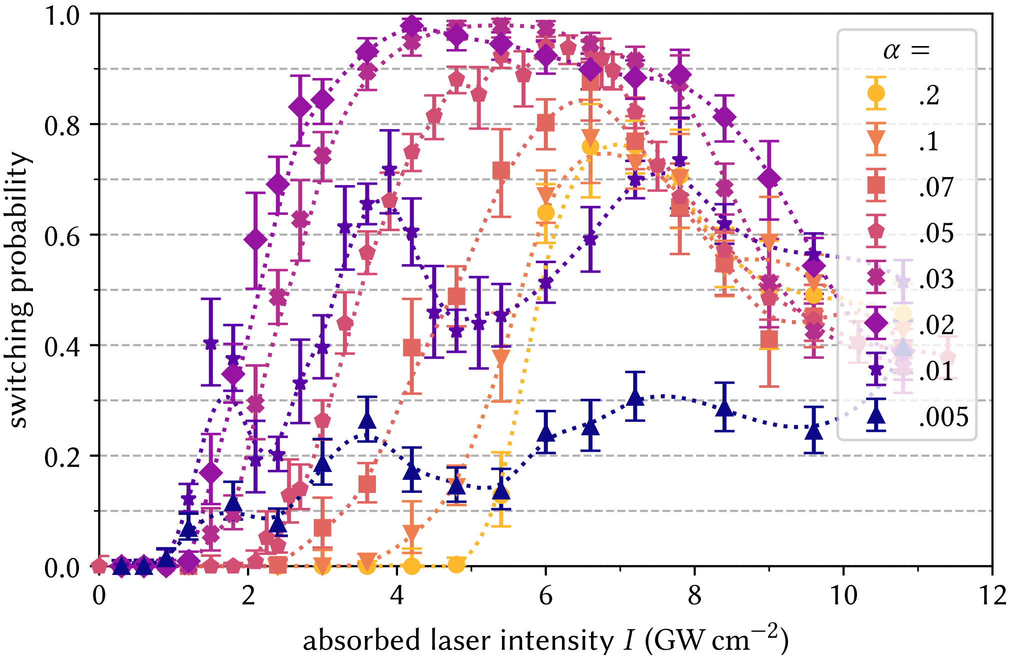


Figure S8: Simulated switching probabilities with different values for the Gilbert damping parameter $\alpha$. The dotted lines serve as a guide to the eye. The error bars indicate the 95 % confidence interval.

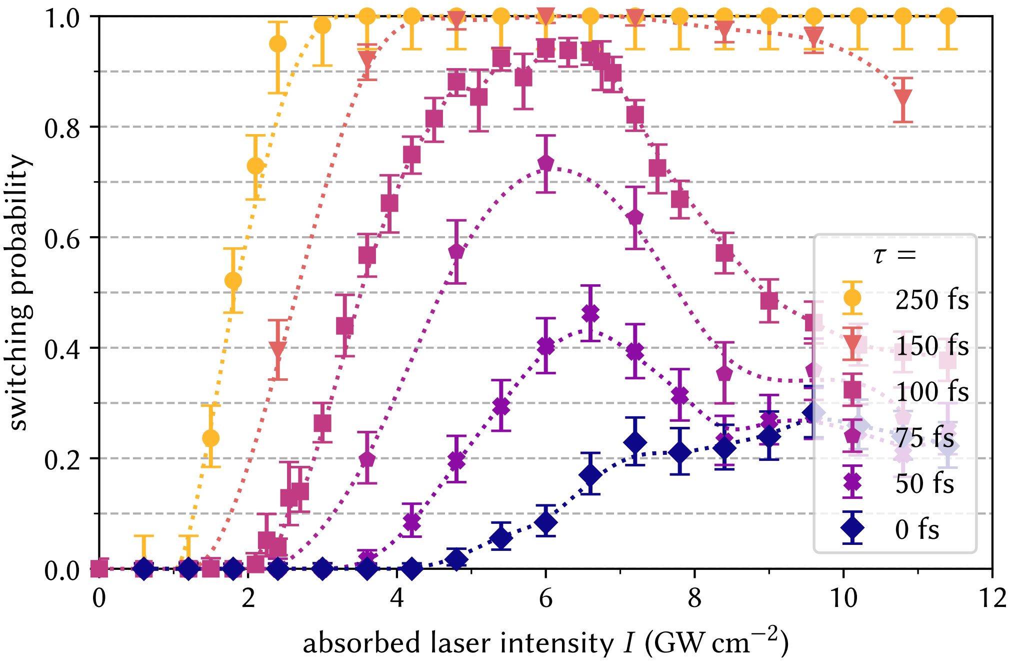


Figure S9: Simulated switching probabilities with different decay times of the induced magnetic moments. The dotted lines serve as a guide to the eye. The error bars indicate the 95 % confidence interval.

diminished for larger values, since the speed of the spin dynamics scales inversely with $\alpha$. For very low damping values, the Néel vector begins to overshoot, which does not facilitate a stable switching process with a deterministic result anymore.

### 2.4 Decay time of the induced moments

For most of the simulations, the decay time $\tau$ of the induced magnetic moments was set to 100 fs. Figure S9 shows the switching probabilities that result from different values of $\tau$. A decay time of around 50 fs seems to be needed at the least to achieve a significant switching probability. For $\tau = 250$ fs, deterministic single-shot switching could be achieved with a wide range of laser intensities.

## References

[1]R. John, M. Berritta, D. Hinzke, C. Müller, T. Santos, H. Ulrichs, P. Nieves, J. Walowski, R. Mondal, O. Chubykalo-Fesenko, J. McCord, P. M. Oppeneer, U. Nowak and M. Münzenberg, 'Magnetisation switching of FePt nanoparticle recording medium by femtosecond laser pulses', Sci. Rep. **7**, 4114 (2017).

[2] I. Radu, K. Vahaplar, C. Stamm, T. Kachel, N. Pontius, H. A. Dürr, T. A. Ostler, J. Barker, R. F. L. Evans, R. W. Chantrell, A. Tsukamoto, A. Itoh, A. Kirilyuk, T. Rasing and A. V. Kimel, 'Transient ferromagnetic-like state mediating ultrafast reversal of antiferromagnetically coupled spins', Nature **472**, 205–208 (2011).

[3] T. A. Ostler, J. Barker, R. F. L. Evans, R. W. Chantrell, U. Atxitia, O. Chubykalo-Fesenko, S. El Moussaoui, L. Le Guyader, E. Mengotti, L. J. Heyderman, F. Nolting, A. Tsukamoto, A. Itoh, D. Afanasiev, B. A. Ivanov, A. M. Kalashnikova, K. Vahaplar, J. Mentink, A. Kirilyuk, T. Rasing and A. V. Kimel, 'Ultrafast heating as a sufficient stimulus for magnetization reversal in a ferrimagnet', Nat. Commun. **3**, 666 (2012).

[4] C. Papusoi, T. Le, C. C. H. Lo, C. Kaiser, M. Desai and R. Acharya, 'Measurements of Gilbert damping parameter $\alpha$ for CoPt-based and CoFe-based films for magnetic recording applications', J. Phys. D **51**, 325002 (2018).

[5] M. Strungaru, S. Ruta, R. F. L. Evans and R. W. Chantrell, 'Model of magnetic damping and anisotropy at elevated temperatures: application to granular FePt films', Phys. Rev. Appl. **14**, 014077 (2020).
